# Supplementary material for: Vibrational Energy Dissipation in Non-Contact Single-Molecule Junctions Governed by Local Geometry and Electronic Structure
Source: arXiv:2504.20791 ancillary file (2025-08-21)
Supplement: Supplementary file 1 [file SI.pdf]

# Supporting Information: Vibrational Energy Dissipation in Single-Molecule Junctions Governed by Local Geometry and Electronic Structure

Lukas Hörmann<sup>\*,†</sup> and Reinhard J. Maurer<sup>\*,†</sup>

<sup>†</sup>*Department of Chemistry, University of Warwick, Gibbet Hill Rd, Coventry, CV4 7AL, United Kingdom*

<sup>‡</sup>*Department of Physics, University of Warwick, Gibbet Hill Rd, Coventry, CV4 7AL, United Kingdom*

E-mail: lukas.hoermann@warwick.ac.uk; r.maurer@warwick.ac.uk

## Contents

|                                                                                      |           |
|--------------------------------------------------------------------------------------|-----------|
| <b>S1 DFT calculations</b>                                                           | <b>2</b>  |
| S1.1 Lattice constant convergence . . . . .                                          | 2         |
| S1.2 K-grid convergence . . . . .                                                    | 2         |
| S1.3 Selecting the functional . . . . .                                              | 3         |
| S1.4 Cu(111) surface geometries . . . . .                                            | 4         |
| S1.5 The Hessian and vibration frequencies of the CO molecule . . . . .              | 5         |
| S1.6 Electron-phonon coupling convergence . . . . .                                  | 7         |
| S1.7 Electronic friction tensors . . . . .                                           | 9         |
| S1.7.1 Electron-phonon coupling of a CO molecule far away from the surface . . . . . | 10        |
| <b>S2 Machine-learned interatomic potentials</b>                                     | <b>11</b> |
| S2.1 Hyperparameter tuning . . . . .                                                 | 11        |
| S2.2 Testing the final potential . . . . .                                           | 13        |
| <b>S3 Lifetimes from different methods</b>                                           | <b>15</b> |
| S3.1 Electron-phonon coupling lifetimes from quasi-harmonic approximation . . . . .  | 15        |
| S3.2 Lifetimes from equilibrium correlation analysis . . . . .                       | 15        |
| S3.3 Lifetimes from explicit dynamics simulations . . . . .                          | 19        |
| S3.4 Comparison of lifetimes from different methods . . . . .                        | 21        |
| <b>S4 Analysis of the velocity cross-correlation function</b>                        | <b>22</b> |
| <b>S5 Coupling strength between vibrational modes</b>                                | <b>23</b> |
| S5.1 Vibrational modes and amplitudes . . . . .                                      | 23        |
| S5.2 Cross-correlation function . . . . .                                            | 26        |
| S5.3 Coupling strength between vibration modes . . . . .                             | 27        |
| <b>References</b>                                                                    | <b>30</b> |

## S1 DFT calculations

For all DFT calculations, we use the FHI-aims quantum chemistry code<sup>1</sup> and numerical atom-centred basis functions. Training data for machine-learned interatomic potentials (MLIP) was created using version 240403, while electron-phonon coupling calculations were done with version 200428.840. Both versions were regression tested to ensure that results were consistent. We first converge the lattice constant. Next, we benchmark functionals with respect to the predicted adsorption site. Then, we compare the computed vibration frequencies to experiment. Finally, we converge the lifetimes resulting from electron-phonon coupling with respect to the numerical settings.

### S1.1 Lattice constant convergence

We converge the lattice constant using a primitive bulk unit cell, with periodic boundary conditions and a k-grid with 24 k-points in each direction. Sweeping the volume around the experimental lattice constant and fitting this data with a Birch–Murnaghan function allows us to determine the lattice constant. We find 2.543 Å and 2.545 Å for PBE+MBD-NL and HSE06+MBD-NL respectively (see Figure S1). For all calculations, we use tight default basis functions.

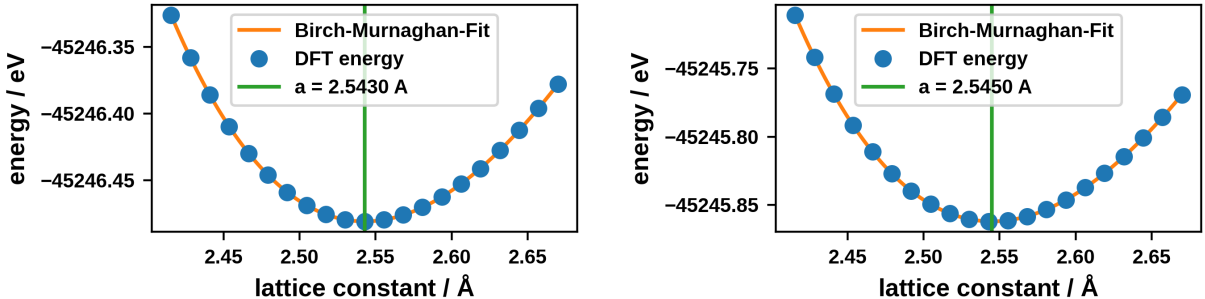

Figure S1: Lattice constant convergence; (left) PBE+MBD-NL; (right) HSE06+MBD-NL

### S1.2 K-grid convergence

Using the lattice constant of 2.543 Å and 2.545 Å for PBE+MBD-NL and HSE06+MBD-NL respectively, we converge the k-grid. We converge the total energy of a bulk Cu crystal since the data with these settings (at HSE06+MBD-NL level) is intended to train MLIPs. Figure S2 shows the k-grid convergence of the total energy. We find that k-grids with 16 and 24 k-points along each reciprocal lattice vector of the primitive bulk unit cell converge the total energy to within 1 meV for PBE+MBD-NL and HSE06+MBD-NL, respectively. Therefore, we use k-grids equivalent to 24 k-points along each reciprocal lattice vector for all HSE06+MBD-NL with periodic boundary conditions.

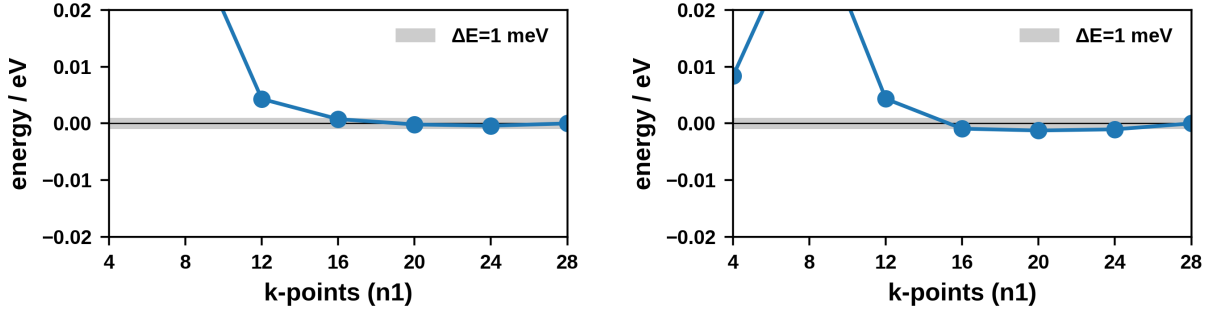

Figure S2: K-grid convergence of the total energy of primitive unit cell of bulk copper; (left) PBE+MBD-NL; (right) HSE06+MBD-NL

### S1.3 Selecting the functional

It is well known that the electronic structure of CO on various metal surfaces is difficult to describe using semi-local DFT.<sup>27,3</sup> In particular, common GGA functionals fail to predict the correct adsorption site, which is attributed to the many-electron self-interaction error. For the present work, it is necessary to use a computation method that yields a qualitatively correct description of the adsorption sites and vibration modes of CO on Cu(111). We test a number of different GGA, meta-GGA, and hybrid functionals in combination with common vdW-correction schemes and compare the computation results to adsorption energies determined using thermal desorption spectroscopy. Table S1 shows that the meta-GGA functional SCAN and the HSE06 short-range separated hybrid functional yield qualitatively correct adsorption energies. We use periodic boundary conditions and the repeated slab approach. The k-grid is equivalent to a (24, 24, 1) k-grid for a primitive surface unit cell.

Table S1: Adsorption energies for CO on Cu(111); \*geometry of HSE06+MBD-NL.

| functional               | adsorption energy / eV                 |            |
|--------------------------|----------------------------------------|------------|
|                          | top                                    | fcc hollow |
| experiment               | -0.46, <sup>4</sup> -0.49 <sup>5</sup> | -          |
| rPBE+vdW <sup>surf</sup> | -0.723                                 | -0.781     |
| PBE+MBD-NL               | -0.967                                 | -1.122     |
| SCAN                     | -1.007                                 | -0.930     |
| HSE06+MBD-NL             | -0.817                                 | -0.761     |
| HSE06*                   | -0.600                                 | -0.536     |

The DFT adsorption energy is an approximation for energies measured with thermal desorption spectroscopy since the DFT energy does not account for zero-point vibrations and finite temperature effects. Therefore, the DFT energies should be seen as upper bounds for the magnitude of the adsorption energy. We included zero-point vibrations for a better comparison to the experiment. Using PBE+MBD-NL, the zero point energies are 0.379 eV and 0.360 eV for the top and fcc-hollow sites, respectively. For HSE06+MBD-NL, the zero-point energies are 0.395 eV and 0.357 eV for the top and fcc-hollow sites, respectively. Accounting for zero-point energies reduces the total binding energy and brings it closer to the experimental values as shown in Table S2. While the energy difference between the top and hollow sites is decreased in both PBE+MBD-NL and HSE06+MBD-NL, the top site remains more energetically favorable in case of HSE06+MBD-NL.

Table S2: Adsorption enthalpies of CO on Cu(111) in eV.

| functional   | adsorption enthalpy / eV               |            |
|--------------|----------------------------------------|------------|
|              | top                                    | fcc hollow |
| experiment   | -0.46, <sup>4</sup> -0.49 <sup>5</sup> | -          |
| PBE+MBD-NL   | -0.588                                 | -0.762     |
| HSE06+MBD-NL | -0.422                                 | -0.404     |

Additionally, we check the site preference for Cu-adatoms (see Table S3) and CO adsorbed on such adatoms (see Table S4) using HSE06+MBD-NL. We find that the fcc-hollow site is preferred over the bridge site, as reported in the literature.<sup>6</sup>

Table S3: Adsorption energy of Cu adatom.

|            | total energy / eV | relative energy / eV |
|------------|-------------------|----------------------|
| fcc hollow | -4388827.986      | 0                    |
| bridge     | -4388827.944      | 0.042                |

Table S4: Adsorption energy of CO on Cu adatom.

|            | total energy / eV | relative energy / eV |
|------------|-------------------|----------------------|
| fcc hollow | -4391913.640      | 0                    |
| bridge     | -4391913.605      | 0.035                |

We find that HSE06+MBD-NL yields qualitatively correct adsorption sites and therefore choose to proceed with this functional.

## S1.4 Cu(111) surface geometries

We consider four surface shapes onto which a CO molecule is placed: A sharp tip, a blunt tip, a (111)-slab with an adatom, and a (111)-slab. All geometries consist of a slab of four Cu layers that act as the base. Onto this slab, the different tip geometries are placed. In the case of the slab and the slab-adatom systems, this base slab is simply continued. The number of layers—counting also adatoms as a layer—of these geometries are given in Table S5.

Table S5: Number of substrate layers for each system.

| system      | unmovable layers | movable layers |
|-------------|------------------|----------------|
| sharp tip   | 4                | 10             |
| blunt tip   | 4                | 0              |
| slab adatom | 4                | 11             |
| slab        | 4                | 10             |

The lattice vectors of the unit cell for the sharp tip and the blunt tip are shown in Listing 1, while those of the slab and slab-adatom systems are shown in Listing 2.

```

1 lattice_vector 30.5159568199999995 0.0000000000000000 0.0000000000000000
2 lattice_vector -15.2579784099999998 26.4275938199999985 0.0000000000000000
3 lattice_vector -0.0000000000000000 -0.0000000000000000 86.2290435999999971

```

Listing 1: Lattice vectors of the sharp tip and blunt tip geometries.

```

1 lattice_vector 15.2579784099999998 0.0000000000000000 0.0000000000000000
2 lattice_vector -7.6289892000000004 13.2137969099999992 0.0000000000000000
3 lattice_vector -0.0000000000000000 -0.0000000000000000 106.9925222699999949

```

Listing 2: Lattice vectors of the slab and slab-adatom geometries.

The four surface geometries contain 795, 793, 505, 504 Cu atoms for the sharp tip, the blunt tip, the slab-adatom, and the slab, respectively. Figure S3 shows the different tip shapes.

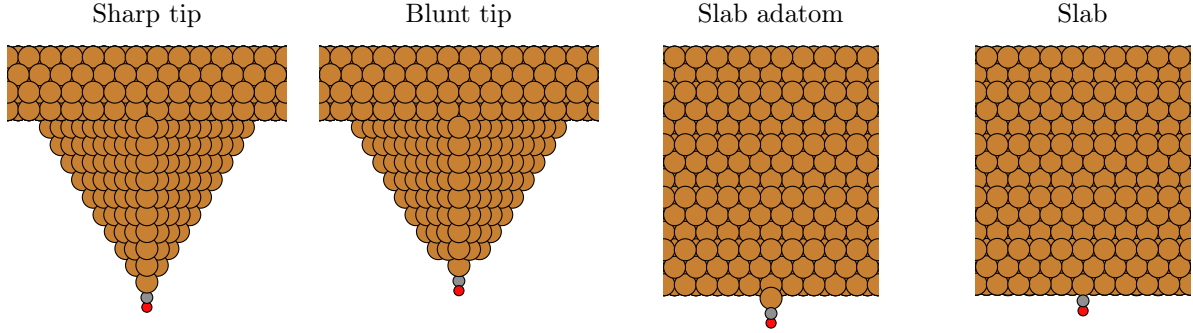

Figure S3: Different tip shapes considered in this study.

### S1.5 The Hessian and vibration frequencies of the CO molecule

CO on different Cu(111) geometries has four vibration modes, which are the frustrated translation (FT), the frustrated rotation (FR), the metal-CO stretch (MS), and the internal stretch (IS). We calculate the vibration frequencies with DFT. We do this to determine the second-order force constants, which are the elements of the Hessian.

$$H_{ij} = \frac{\partial^2 V}{\partial x_i \partial x_j} \quad (1)$$

Figure S4 shows a row in the Hessian, i.e.  $H_{ij}$  for a fixed  $i$ . The index  $i$  was chosen to be the x-axis degree of freedom of the C atom. The degrees of freedom are in no particular order. Each panel shows a different tip shape. The bars indicate the absolute value of the element  $H_{ij}$ . Large elements indicate strong coupling between the respective degrees of freedom.

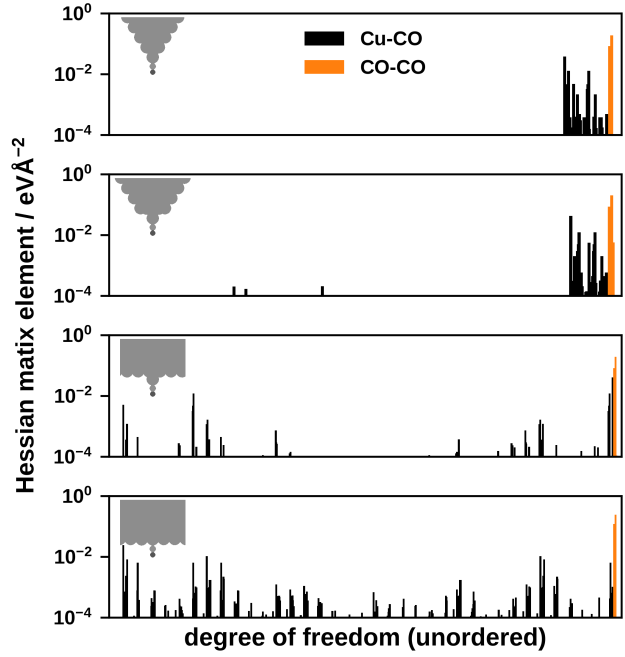

Figure S4: Off-diagonal elements of the Hessian.

Calculated vibrational frequencies are shown in Tables S7 and S8 for PBE+MBD-NL as well as HSE06+MBD-NL, respectively. Table S6 shows vibration frequencies determined by hydrogen scattering<sup>7</sup> and infrared spectroscopy.<sup>8</sup> The comparison of the three tables shows that PBE+MBD-NL and HSE06+MBD-NL yield vibrational frequencies for these modes that agree well with experiment.

Table S6: Vibration frequencies of CO molecule on a surface from experiment.

|                     | vibrational energy / meV |       |       |        |
|---------------------|--------------------------|-------|-------|--------|
|                     | FT                       | FR    | MS    | IS     |
| slab <sup>7,8</sup> | 4.07                     | 36.47 | 41.41 | 257.63 |

Table S7: Vibration frequencies of CO molecule on different geometries at PBE+MBD-NL level.

|                 | vibrational energy / meV |       |       |        |
|-----------------|--------------------------|-------|-------|--------|
|                 | FT                       | FR    | MS    | IS     |
| sharp tip       | 3.25                     | 31.69 | 49.51 | 254.80 |
| blunt tip       | 3.56                     | 34.23 | 51.13 | 254.68 |
| slab top        | 5.29                     | 35.46 | 47.87 | 250.19 |
| slab fcc hollow | 18.14                    | 30.55 | 37.95 | 224.62 |

Table S8: Vibration frequencies of CO molecule on different geometries at HSE06+MBD-NL level.

|                 | vibrational energy / meV |       |       |        |
|-----------------|--------------------------|-------|-------|--------|
|                 | FT                       | FR    | MS    | IS     |
| sharp tip       | 2.9                      | 29.07 | 45.44 | 271.97 |
| blunt tip       | 2.94                     | 31.21 | 45.63 | 272.16 |
| slab adatom     | 3.27                     | 32.57 | 45.32 | 274.12 |
| slab top        | 5.49                     | 36.5  | 44.68 | 266.21 |
| slab fcc hollow | 14.32                    | 24.86 | 34.37 | 243.88 |

## S1.6 Electron-phonon coupling convergence

To calculate electron-phonon coupling, we use a blunt Cu-tip placed on a Cu-slab made up of four layers. We use periodic boundary conditions and the repeated slab approach, with a dipole correction. The unit cell contains 144 slab surface atoms and has the following lattice vectors:

|   |                             |              |             |             |
|---|-----------------------------|--------------|-------------|-------------|
| 1 | <code>lattice_vector</code> | 30.51595682  | 0.00000000  | 0.00000000  |
| 2 | <code>lattice_vector</code> | -15.25797841 | 26.42759382 | 0.00000000  |
| 3 | <code>lattice_vector</code> | 0.00000000   | 0.00000000  | 86.22904360 |

We converge the number of atom layers and the number of k-points. For Cu-atoms, we use light default basis functions, while we use tight defaults for all other species. Figure S5 shows the convergence of the number of layers in the tip with respect to the lifetime of the four non-degenerate vibration modes of the CO molecule adsorbed on the sharp Cu-tip. The number of layers in the slab is always four, and all calculations use the same unit cell. The convergence shows us that four slab layers + 9 layers in the Cu-tip are sufficient to converge the lifetime of the vibration modes.

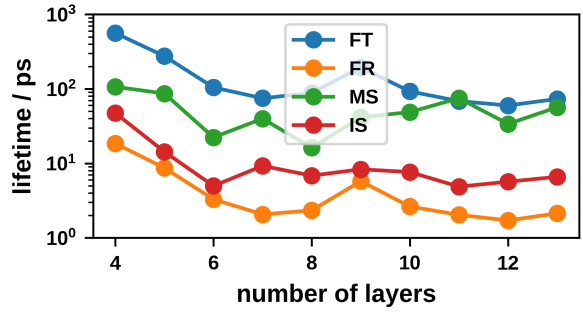

Figure S5: Layer convergence of the lifetime of the different CO vibration modes as a result of electron-phonon coupling for CO on a blunt tip

Figure S6 shows the convergence of the k-grid with respect to the lifetime of the non-degenerate vibration modes of the CO molecule on a surface slab. We use a (6, 6) unit cell to ensure that the CO molecule does not interact with its image. We test two different friction broadening values of 0.1 eV and 0.3 eV (default setting). We find that a k-grid of (24, 24, 1) for the primitive substrate unit cell converges the lifetime. In the case of the (6, 6) unit cell, this k-grid would correspond to (4, 4, 1) k-points. Moreover, the default broadening of 0.3 eV shows better k-grid convergence.

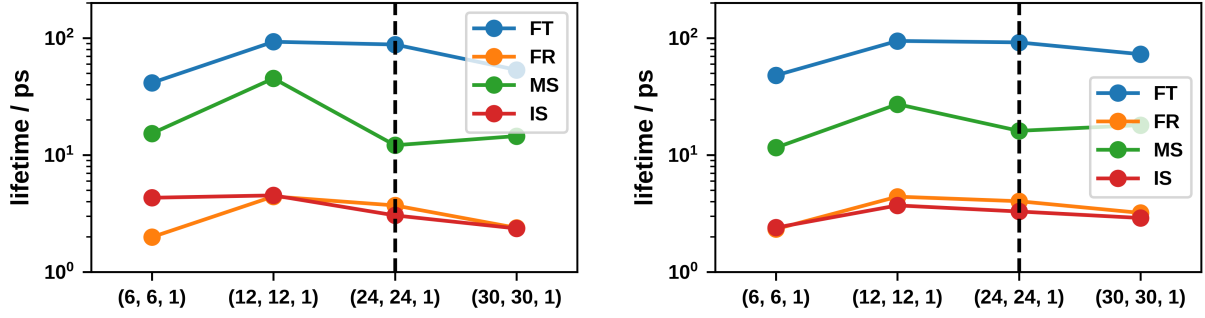

Figure S6: K-point convergence of the lifetime of the different CO vibration modes as a result of electron-phonon coupling for CO on a Cu(111) slab; left) friction broadening 0.1 eV; right) friction broadening 0.3 eV.

Figure S6 also shows better k-point convergence for a broadening of 0.3 eV. To gauge the effect of the friction broadening, we sweep the broadening in Figure S7. The broadening should be chosen as small as possible. We find that broadening values larger than the default of 0.3 eV do not significantly affect the lifetimes.

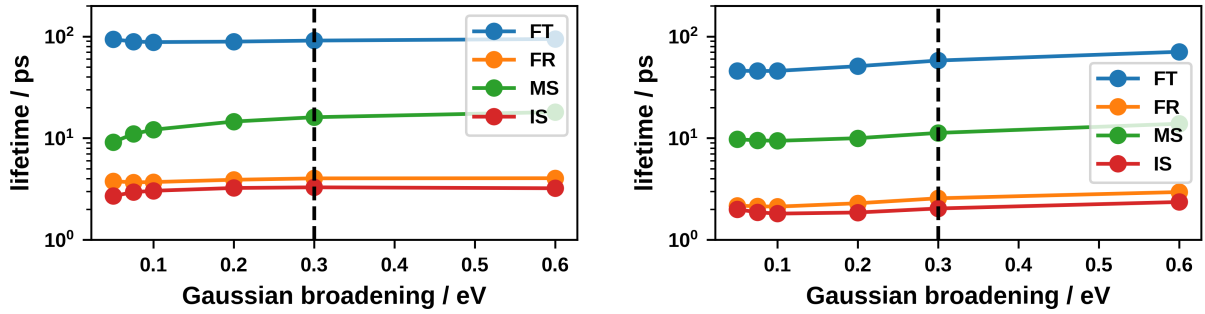

Figure S7: Dependence of the lifetime of the different CO vibration modes as a result of electron-phonon coupling for CO on a slab on the friction broadening; the k-grid is (24, 24, 1) for the primitive substrate unit cell; left) perturbing frequency of zero; right) perturbing frequency of the respective IS mode.

Below, is a control file for the converged settings to calculate electron friction for the surface slab:

```

1  # General Settings:
2  xc                               pbe
3  spin                             none
4  charge                           0.0
5  relativistic                     atomic_zora scalar
6  occupation_type gaussian         0.01
7  k_grid                           4 4 1
8
9  # Convergence Criteria:
10 sc_accuracy_etot                  1e-06
11 sc_accuracy_eev                   1e-03
12 sc_accuracy_rho                   1e-05
13 sc_iter_limit                     200
14
15 # Other Settings:

```

```

16 use_dipole_correction      # friction_tensor in 1/ps
17 # n_atom 1 i_cart 1 index 1
18     0.014283   -0.000002   -0.000000
19 # n_atom 1 i_cart 2 index 2
20     -0.000002    0.014285   -0.000001
21 # n_atom 1 i_cart 3 index 3
22     -0.000000   -0.000001    0.014281   .true.
23 compensate_multipole_errors .true.
24
25 # Friction keywords
26 calculate_friction          numerical_friction
27 friction_numeric_disp      0.001
28 friction_broadening_width  0.3
29 friction_temperature       5
30 friction_delta_type        gaussian
31 output_friction_eigenvectors .true.
32 friction_iter_limit        100
33 calculate_all_eigenstates
34 friction_delta_normalisation .false.
35 friction_max_energy        2.4

```

## S1.7 Electronic friction tensors

The entire electronic friction tensor is approximated by combining a friction tensor calculated for a CO molecule adsorbed on the Cu surface with friction values calculated for the Cu bulk. For the Cu atoms, we use a diagonal electronic friction tensor, where electronic is homogeneous in all directions. The friction tensor for the adsorbed CO molecule is shown in Listing 3. The friction value for the Cu atoms is determined by calculating the electronic friction tensor for a Cu atom in the middle of a 5x5x5 Cu bulk unit cell. This electronic friction tensor is shown in Listing 4 and displays similar electronic friction coefficients in each degree of freedom.

```

1 # friction_tensor in 1/ps
2 # n_atom 505 i_cart 1 index 1
3     0.026131   -0.000003   -0.000003   -0.076470   -0.000009   0.000036
4 # n_atom 505 i_cart 2 index 2
5     -0.000003    0.026078    0.000052    0.000009   -0.076360   0.000049
6 # n_atom 505 i_cart 3 index 3
7     -0.000003    0.000052    0.055054    0.000074   -0.000071   -0.099630
8 # n_atom 506 i_cart 1 index 4
9     -0.076470    0.000009    0.000074    0.229697    0.000005   -0.000213
10 # n_atom 506 i_cart 2 index 5
11     -0.000009   -0.076360   -0.000071    0.000005    0.229491   -0.000015
12 # n_atom 506 i_cart 3 index 6
13     0.000036    0.000049   -0.099630   -0.000213   -0.000015    0.313573

```

Listing 3: CO molecule adsorbed on the Cu(111) slab.

```

1 # # friction_tensor in 1/ps
2 # n_atom 1 i_cart 1 index 1
3     0.014283   -0.000002   -0.000000
4 # n_atom 1 i_cart 2 index 2

```

```

5      -0.000002      0.014285      -0.000001
6 # n_atom  1 i_cart  3 index  3
7      -0.000000      -0.000001      0.014281

```

Listing 4: Cu atom in Cu bulk.

### S1.7.1 Electron-phonon coupling of a CO molecule far away from the surface

We compare the electronic friction tensor of a CO molecule adsorbed on the Cu(111) slab to that of the CO molecule approximately 5 Å away from the slab. The adsorbed system, shown in Listing 3, shows electronic friction coefficients that are four orders of magnitude larger than the system where the molecule is at a distance, shown in Listing 5.

```

1  # friction_tensor in 1/ps
2 # n_atom 505 i_cart  1 index  1
3      0.000002      0.000000      -0.000000      -0.000000      0.000001      -0.000001
4 # n_atom 505 i_cart  2 index  2
5      0.000000      0.000001      -0.000000      0.000000      -0.000000      -0.000000
6 # n_atom 505 i_cart  3 index  3
7      -0.000000      -0.000000      0.000093      -0.000000      0.000000      -0.000105
8 # n_atom 506 i_cart  1 index  4
9      -0.000000      0.000000      -0.000000      0.000002      0.000000      -0.000001
10 # n_atom 506 i_cart  2 index  5
11      0.000001      -0.000000      0.000000      0.000000      0.000003      -0.000001
12 # n_atom 506 i_cart  3 index  6
13      -0.000001      -0.000000      -0.000105      -0.000001      -0.000001      0.000124

```

Listing 5: CO molecule at a distance of 5 Å away from the Cu(111) slab.

## S2 Machine-learned interatomic potentials

We use the MACE potential,<sup>9</sup> version 0.3.4, which is an equivariant neural-network potential. The training, test, and validation sets were chosen from a dataset containing 621 calculations performed at the HSE06+MBD-NL level of theory. This dataset includes structures sampled from molecular dynamics (MD) simulations using lower-accuracy MLIPs, configurations with randomly perturbed atomic positions, structures obtained during geometry optimisation, and vibration calculations. The structures in the training set range from 79 Cu atom clusters to a CO molecule adsorbed on a 796-atom Cu surface geometry. To find the best potential, we determine the optimal cutoff distance ( $r_{\text{max}}$ ) and the message size (hidden\_irreps). For each combination of cutoff distance and message size, we train five potentials, evaluate the training and validation errors, and determine the mean value of these errors. Figures S8 and S9 show the results for energies and forces, respectively. Because these MLIPs are intended to run MD simulations, we place greater emphasis on accurate forces when selecting the parameters.

### S2.1 Hyperparameter tuning

We perform a hyperparameter search to find optimal model parameters that deliver minimal root mean square errors (RMSE) and mean absolute errors (MAE) on the test set and provide robust models in terms of cross-validation. We test different combinations of cutoff distance ( $r_{\text{max}}$ ) and the message size (hidden\_irreps). For each combination of cutoff distance and message size, we trained five potentials, evaluated the training and validation errors, and determined the mean value of these errors. For this, we use k-fold cross-validation, where we split our dataset into five equally sized segments. Four segments are used for training, while the final segment is split into a validation and a test set. We use the validation set for hyperparameter selection. Figures S8 and S9 show the averaged errors for energies and forces, respectively. Because these MLIPs are intended to run MD simulations, we place greater emphasis on accurate forces when selecting the parameters.

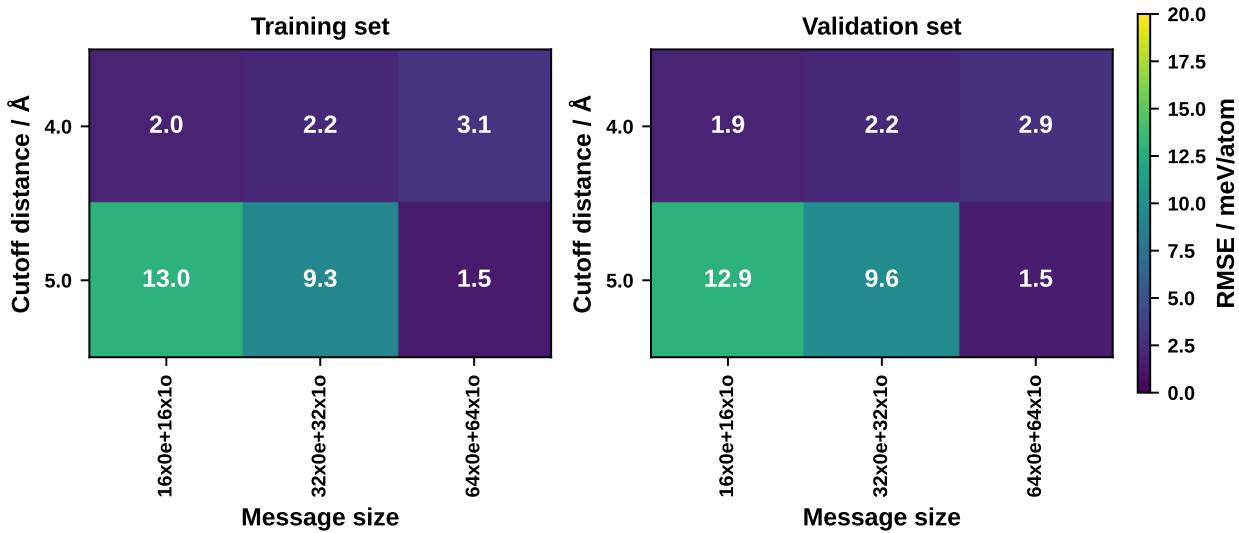

Figure S8: Average energy error for different MACE potentials.

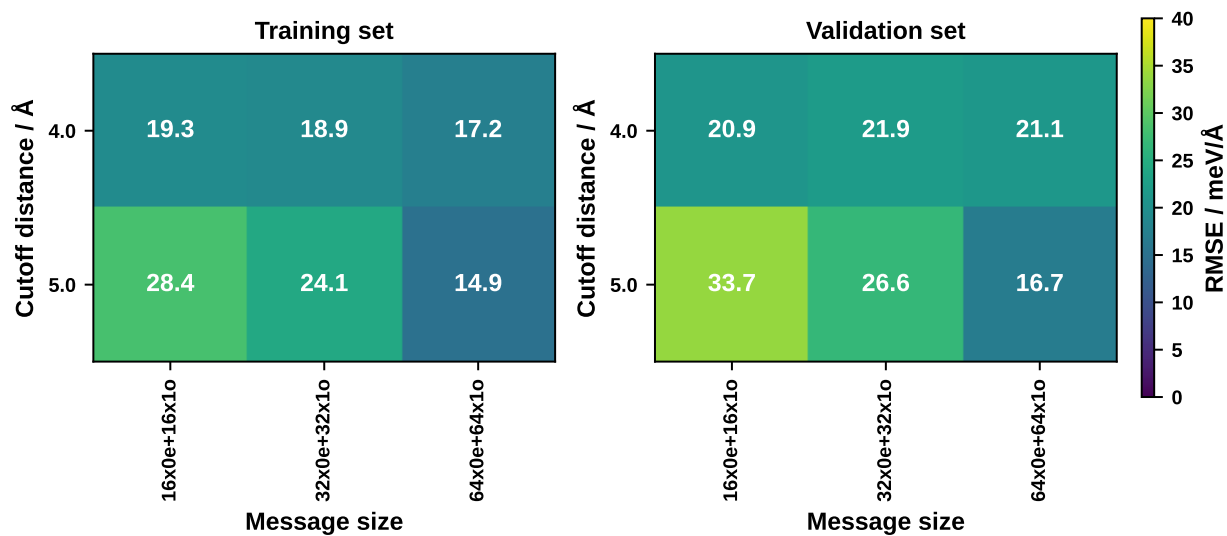

Figure S9: Average force error for different MACE potentials.

When analysing the force errors in Figure S10, we find that a cutoff radius 4.0 Å or 5.0 Å leads to the smallest training and validation set errors. Moreover, the errors decrease with increasing message size. To select the final production training set, we determine the potentials with the lowest training and validation errors. Figure S10 shows the potential with the smallest force error for each combination of parameters.

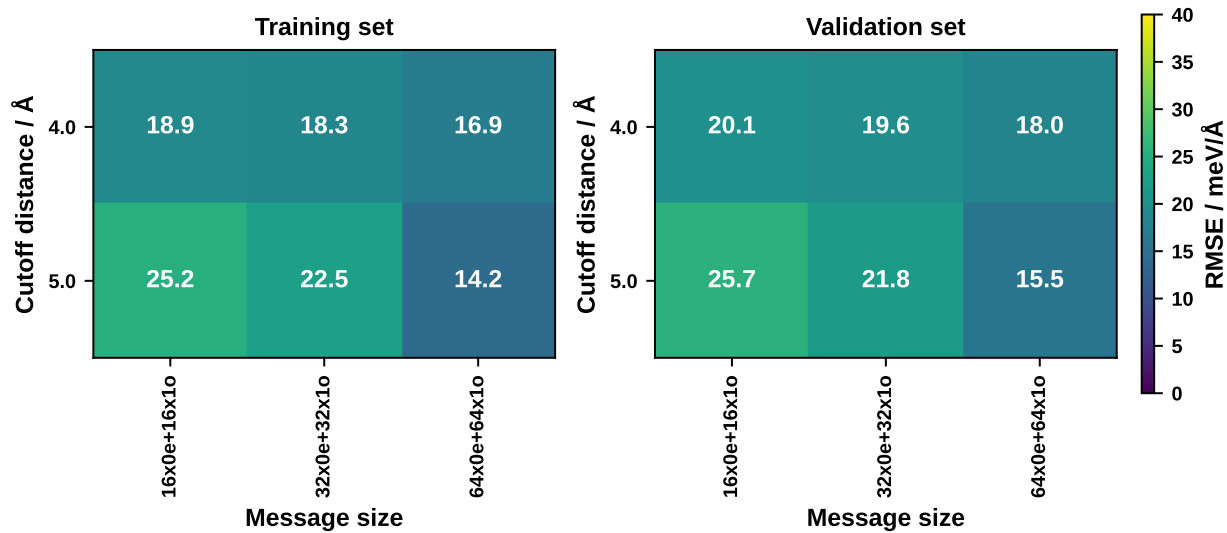

Figure S10: Smallest force errors achieved for each combination of cutoff distance and the message size.

We find that a cutoff radius of 5.0 Å combined with a message size of 64x0e + 64x1o yields the best MLIP. The following code section shows the final parameters for the MACE potential.

```

1  name = MACE_model
2  train_file = data/train.xyz
3  valid_file = data/valid.xyz
4  test_file = data/test.xyz
5  config_type_weights = {"Default":1.0}
6  EOs = {6:-0.102674349116667E+04, 8:-0.203970920939905E+04, 29:-0.452419011191033E+05}
7  model = MACE
8  hidden_irreps = 64x0e+64x1o
9  r_max = 5.0
10 batch_size = 10
11 max_num_epochs = 1500
12 swa = True
13 start_swa=1200
14 ema = True
15 ema_decay=0.99
16 amsgrad = True
17 restart_latest = True
18 device = cuda
19 save_cpu = True
20 forces_weight = 95
21 swa_forces_weight = 1
22 energy_weight = 5
23 swa_energy_weight = 10
24 correlation = 2
25 num_interactions = 2
26 num_radial_basis = 3
27 num_cutoff_basis = 4
28 default_dtype = float64

```

Using the five training, test, and validation sets described earlier, we quantified uncertainties on the test set based on the final model parameters (a cutoff radius of 5.0 Å and a message size of 64x0e + 64x1o). Table S9 presents the average errors across the five sets for all atoms, along with the force errors specifically for the O atom in the CO molecule and the Cu atoms.

Table S9: Averaged errors for energies and forces for five different samples.

| Species | Energy / meV/atom |                  | Force / meV Å <sup>-1</sup> |                   |
|---------|-------------------|------------------|-----------------------------|-------------------|
|         | RMSE              | MAE              | RMSE                        | MAE               |
| Cu      | -                 | -                | 15.7 (2.0)                  | 10.0 (0.9)        |
| O       | -                 | -                | 32.6 (9.3)                  | 16.8 (3.8)        |
| All     | <b>1.6 (0.2)</b>  | <b>1.2 (0.2)</b> | <b>15.9 (1.9)</b>           | <b>10.0 (0.9)</b> |

## S2.2 Testing the final potential

As the final model, we chose the model that yielded the smallest force error in Figure S10. To test the accuracy of our final MACE potential, we determine learning curves for energies and forces, which are shown in Figure S11. Potentials were trained using training sets containing 150, 200, 250, 300, 350, 400, 450, and 504 calculations. The smaller training sets were randomly selected from the set of 504 data points. The training was done using a validation set containing 69 calculations. We evaluated all models on the test set containing 48 calculations. As expected, larger training sets lead to a clear improvement in prediction

accuracy across all data sets, and we are therefore confident in the validity of our final MACE potential. The errors of the final potential trained on 504 data points are shown in Table S10.

Table S10: Errors for energies and forces for the final potential trained on 504 data points.

| Species    | Energy / meV/atom |            | Force / meV Å <sup>-1</sup> |            |
|------------|-------------------|------------|-----------------------------|------------|
|            | RMSE              | MAE        | RMSE                        | MAE        |
| Cu         | -                 | -          | 15.6                        | 9.6        |
| O          | -                 | -          | 27.7                        | 16.2       |
| <b>All</b> | <b>2.0</b>        | <b>1.6</b> | <b>15.7</b>                 | <b>9.6</b> |

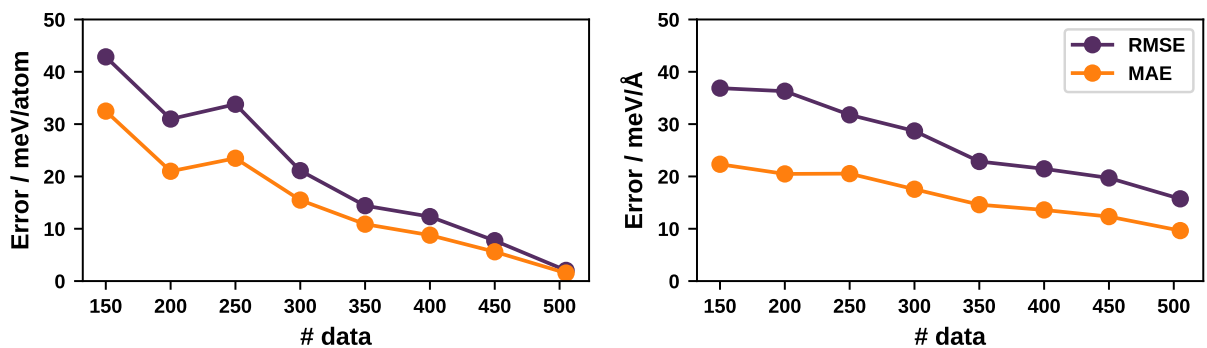

Figure S11: Learning curve for the final MACE potential

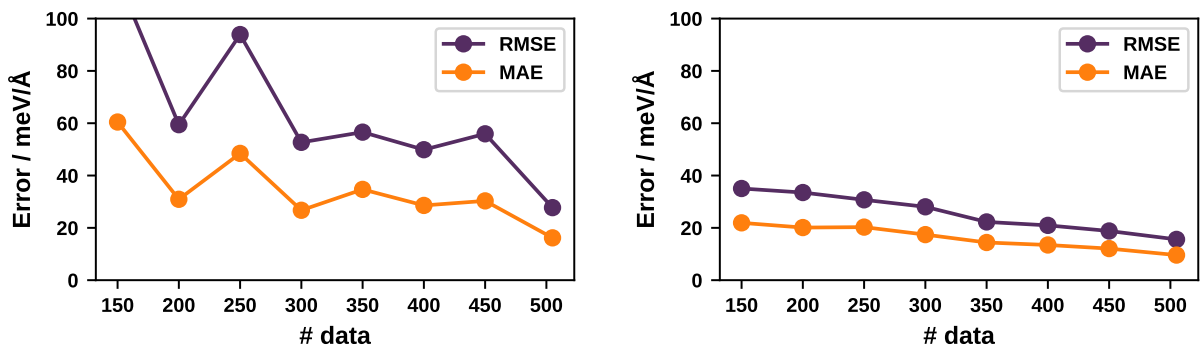

Figure S12: Learning curve for left) O-atoms; right) Cu-atoms

## S3 Lifetimes from different methods

### S3.1 Electron-phonon coupling lifetimes from quasi-harmonic approximation

To demonstrate the impact of the finite perturbation frequency on electron-phonon coupling lifetimes determined through the first-order perturbation theory and the quasi-harmonic approximation, we compare the case with zero perturbation frequency (Table S11) to that with a finite perturbation frequency (Table S12) given by the frequency of the respective vibration mode.

Table S11: Electron-phonon lifetimes using zero perturbing frequencies.

|             | Lifetime / ps |      |      |     |
|-------------|---------------|------|------|-----|
|             | FT            | FR   | SA   | IS  |
| sharp tip   | 187.7         | 24.7 | 93.6 | 7.7 |
| blunt tip   | 102.3         | 6.5  | 44.8 | 6.5 |
| slab adatom | 116.2         | 11.8 | 60.5 | 9.3 |
| slab        | 63.8          | 4.0  | 13.8 | 3.1 |

Table S12: Electron-phonon lifetimes using finite perturbing frequencies.

|             | Lifetime / ps |      |      |     |
|-------------|---------------|------|------|-----|
|             | FT            | FR   | SA   | IS  |
| sharp tip   | 185.9         | 21.2 | 80.0 | 2.8 |
| blunt tip   | 99.1          | 6.0  | 39.0 | 3.3 |
| slab adatom | 110.8         | 10.8 | 52.9 | 4.9 |
| slab        | 47.9          | 3.6  | 12.5 | 1.9 |

### S3.2 Lifetimes from equilibrium correlation analysis

**Convergence of the length of molecular dynamics trajectories.** We converge the lifetimes of the CO-vibration modes—frustrated translation (FT), frustrated rotation (FR), surface adsorbate stretch (SA), and internal stretch (IS)—with respect to the length of the MD-trajectories. We consider two cases: (A) regular molecular dynamics, where the lifetime is a result of phonon-phonon coupling (phononic friction), and (B) non-adiabatic molecular dynamics, where the lifetime is a result of electron-phonon and phonon-phonon coupling. To determine the lifetimes, we used normal mode decomposition and analysis of the velocity cross-correlation function via the Welch method (see Section S4). Figure S13 shows the convergence for the different surface geometries and vibration modes for the case where we have only phonon-phonon coupling. Using the standard deviation of the lifetime for the final three trajectory lengths, we find that a length of approximately 2000 ps converges the lifetime to an uncertainty of below 15%. We note that the convergence for the FT mode of the slab shows a larger standard deviation on the final three lengths. We consider this result converged since we do not see an increase in lifetime.

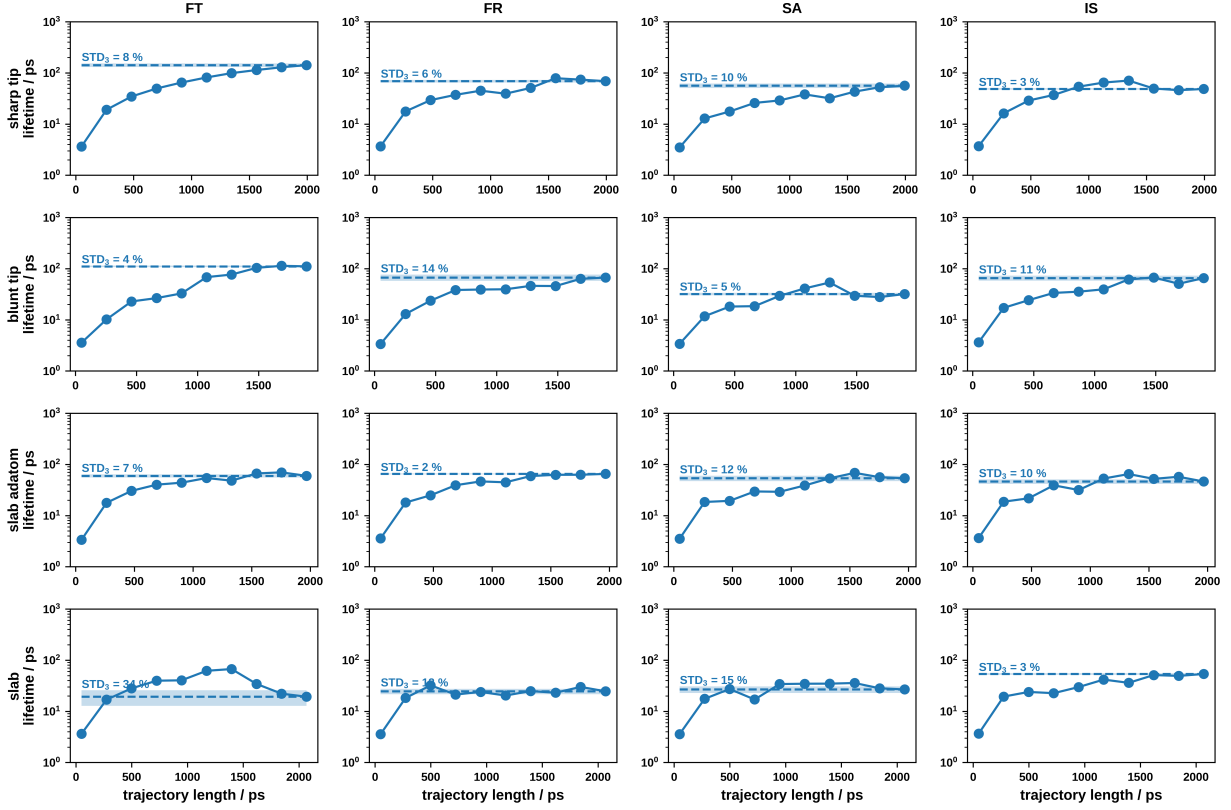

Figure S13: Convergence of CO vibrational lifetimes with respect to trajectory length; Lifetime resulting from electron-phonon and phononic coupling.

For the case where phonon-phonon and electron-phonon coupling affect the lifetimes—calculated with molecular dynamics with electronic friction (MDEF)—the convergence for the different surface geometries and vibration modes is shown in Figure S14. Due to the increased dampening due to electron-phonon coupling, vibrational lifetimes are shorter than in the case where only phonon-phonon coupling is active. This leads to better convergence. The standard deviation of the lifetime for the final three trajectory lengths shows that a length of approximately 900 ps converges the lifetime to an uncertainty of below 15 %.

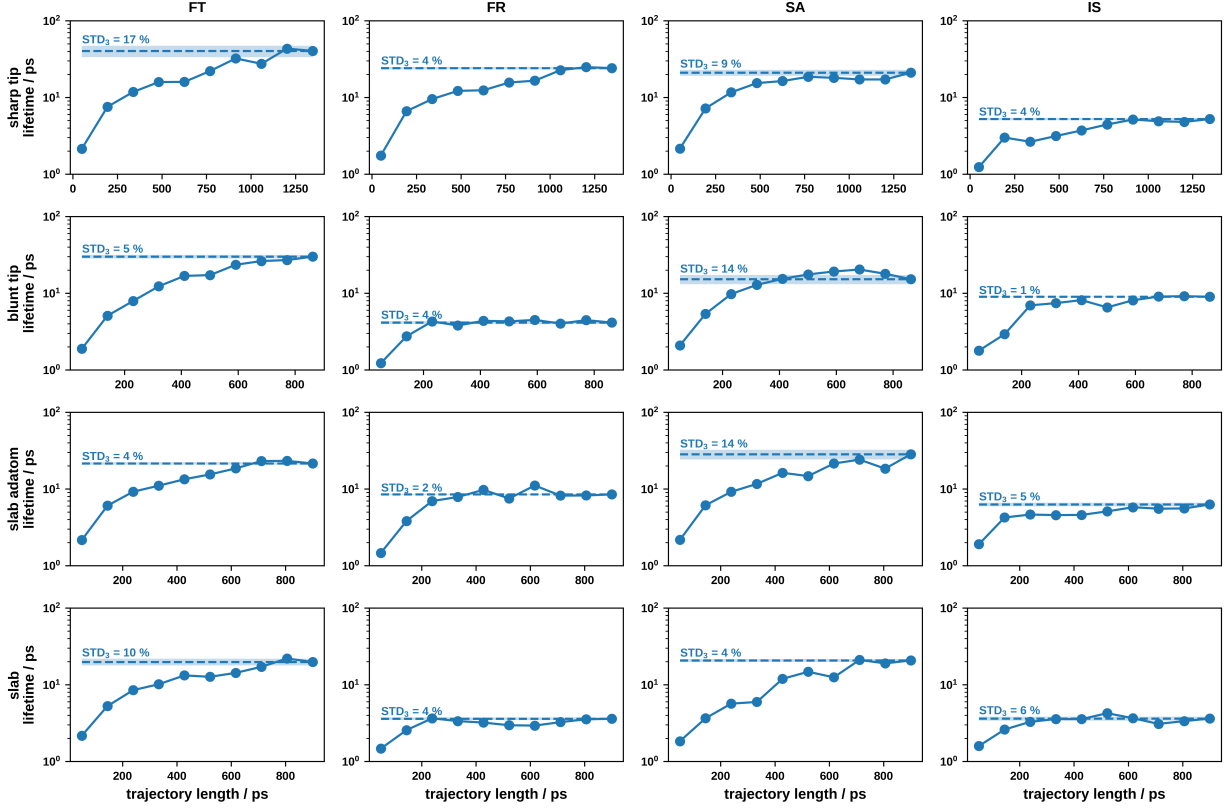

Figure S14: Convergence of CO vibrational lifetimes with respect to trajectory length; Lifetime resulting from phononic coupling.

The final values of the convergence curves for trajectory length in Figures S13 and S14 are taken as the lifetime, and the standard deviation over the last three convergence steps is taken as the uncertainty. Lifetimes determined via equilibrium correlation analysis are shown in Chapter S3.4.

**Examples of the power-spectrum and the cross-spectrum.** As we explain in the results chapter on phonon-phonon coupling in the main manuscript, we determine lifetimes based on equilibrium dynamics by analyzing the cross-spectrum. This is the Fourier transform of the velocity cross-correlation function. The cross-spectrum  $\tilde{C}_{ij}(\omega)$  represents the coupling between the vibration modes  $i$  and  $j$ . Its diagonal elements  $\tilde{C}_{ii}(\omega)$  contain one peak at the characteristic frequency of the mode  $i$ , whose width corresponds to the lifetime. The diagonal elements of the cross-spectrum are called the power spectrum and are exemplarily shown for the blunt tip in Figure S15.

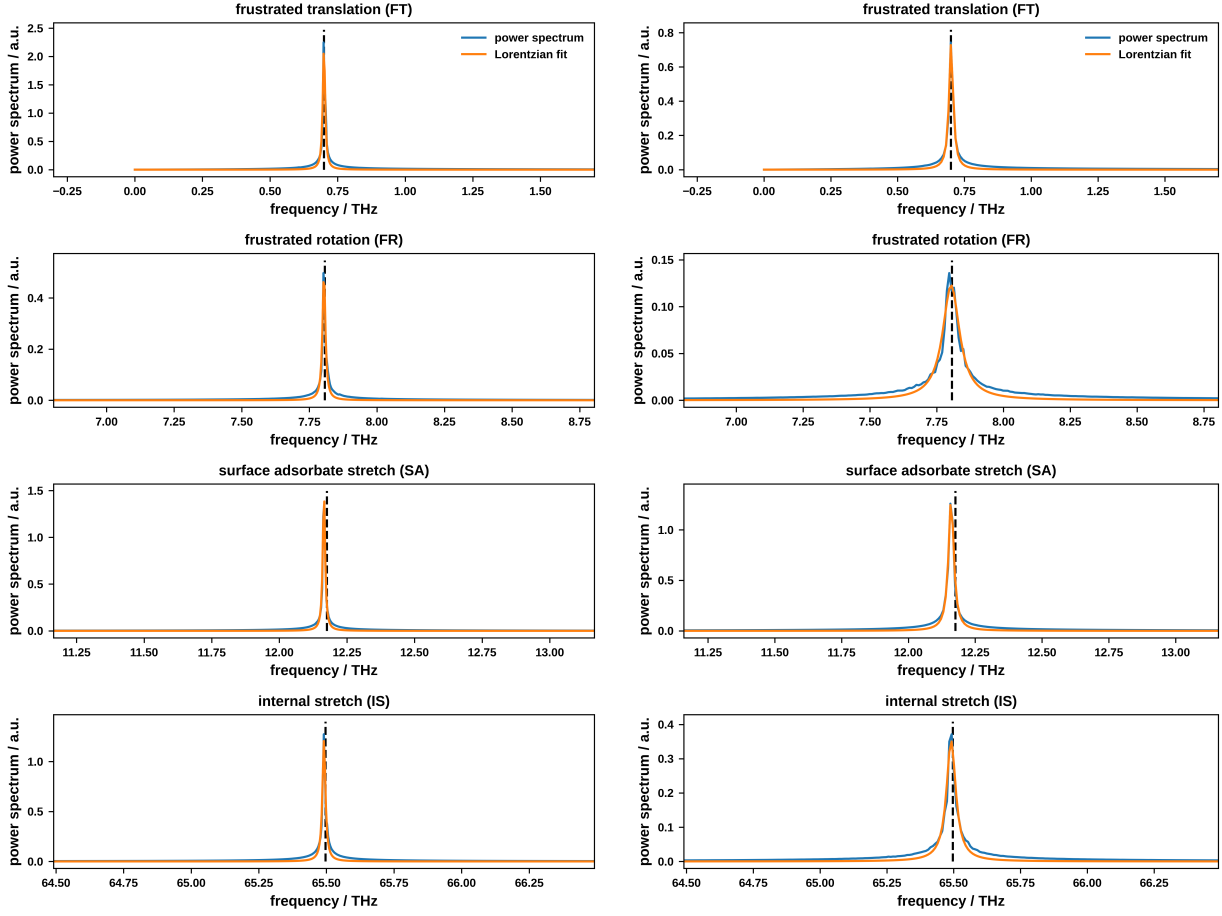

Figure S15: Power spectra of the different CO modes of the blunt tip; Left) only with phonon-phonon coupling; Right) with electron-phonon and phonon-phonon coupling.

Its off-diagonal elements  $\tilde{C}_{ij}(\omega)$  show two peaks at the characteristic frequencies of the two vibration modes  $i$  and  $j$ . An example of the cross-spectrum between the FT and the RF mode of the CO molecule is shown in Figure S16. We note that in our work, the cross-spectrum contains all coupling between CO and metal modes.

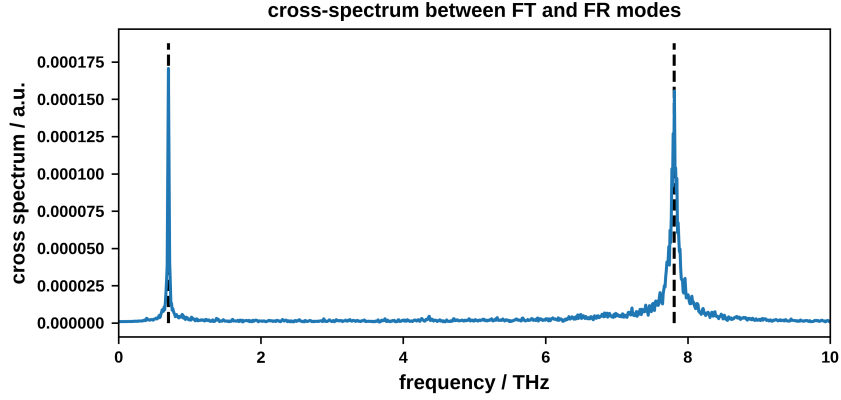

Figure S16: Cross spectrum of the different FT and FR modes of the blunt tip.

### S3.3 Lifetimes from explicit dynamics simulations

We analyze the effect of activation energy by exciting the FT mode with 50 meV, 100 meV, and 200 meV. The results are shown in Figure S17. The FT mode exhibits harmonic behavior at 50 meV and remains harmonic at even higher energies when influenced by a sharp tip or a slab. Since 50 meV is large compared to the vibrational energy of the FT mode (approximately 5 meV), increasing the activation energy introduces significant anharmonicity-related effects on the lifetimes. This effect is most pronounced for the blunt tip and the slab-adatom, where a large activation energy leads to non-harmonic behavior. In contrast, for the FT mode of the sharp tip and the slab, lifetimes remain robust against changes in activation energy.

Due to anharmonicity, other modes are also activated, with the largest secondary activation occurring in the IS mode. The lifetimes of the IS mode are generally stable across different activation energies, except for very small activation energies, as observed for the IS mode of the slab. The SA mode also experiences significant secondary activation and exhibits a robust lifetime. On the slab, however, the secondary activation energy is too low, causing the decay to be lost in thermal noise and the inherent uncertainty of the simulations. The FR mode receives only minor secondary activation, with only the sharp tip providing sufficient energy to determine lifetimes. Overall, we find that the activation energy must strike a balance: it should be large enough to produce a measurable decay but small enough to minimize anharmonicity effects. Our results indicate that 50 meV achieves this balance.

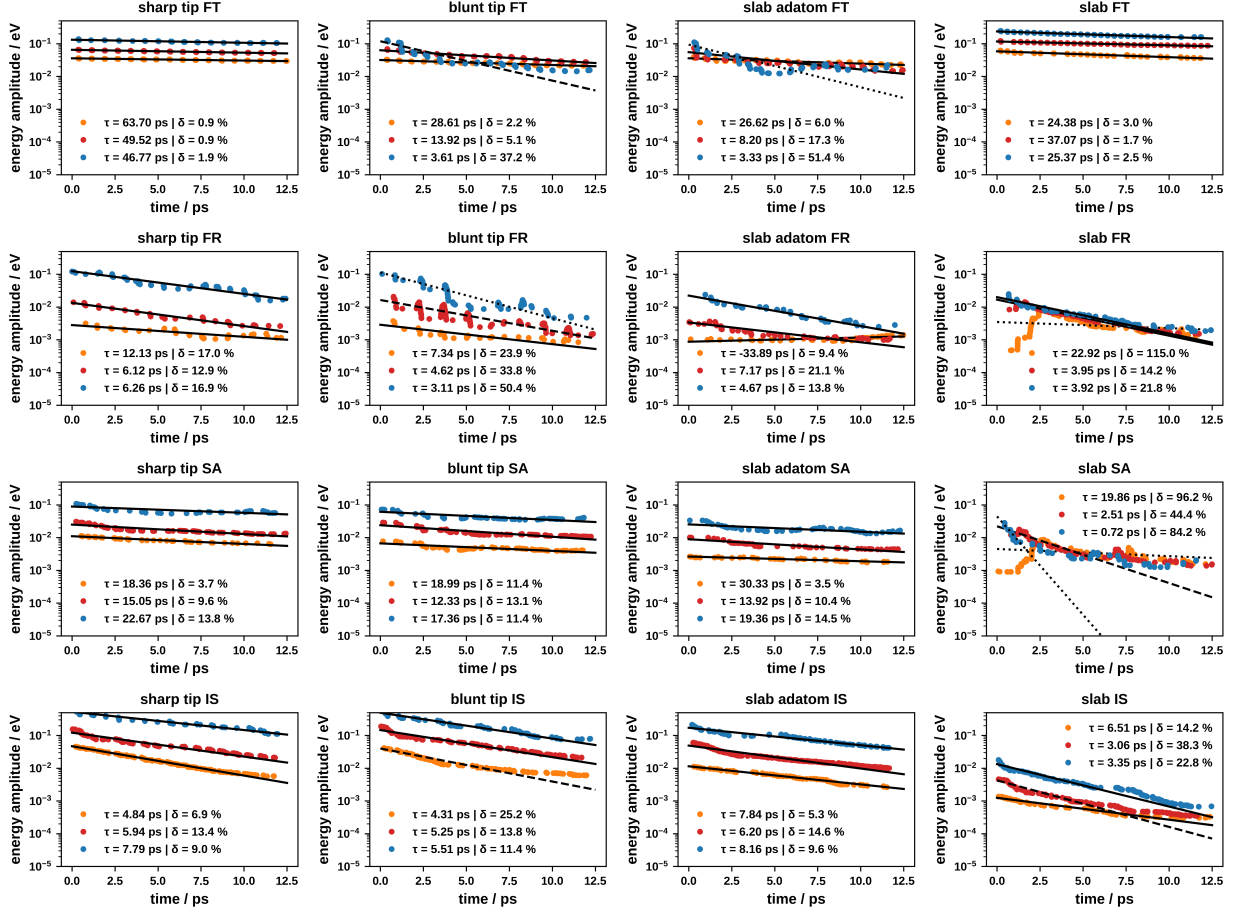

Figure S17: Energy dissipation in of the four CO-modes, when the FT mode is activated with 50 meV (orange), 100 meV (red), and 200 meV (blue) of energy.

The analysis of the secondary activation of other CO modes in Figure S17 provides insight into the anharmonicity of different systems. Secondary activation energies, which serve as an indicator of anharmonicity, decrease as the substrate geometry becomes flatter. A large secondary activation indicates strong anharmonicity. Therefore, we conclude that the sharp tip is the most anharmonic system, while the slab is the most harmonic.

To determine the production lifetime from explicit dynamic simulations, we conduct 64 simulations, each starting with randomised initial velocities at a temperature of 5 K. The system is then thermalised at 5 K for 50,000 MD(EF) steps. As in all dynamic simulations in this work, we use a time step of 0.1 fs. After thermalisation, we activate the CO mode of interest with 50 meV and monitor the decay of the kinetic energy envelope. Performing this analysis over 64 trajectories allows us to determine robust lifetimes, which are compared to other lifetimes from other methods in Chapter S3.4.

### S3.4 Comparison of lifetimes from different methods

Phonon-phonon lifetimes are calculated in two different ways (see Table S13). We attribute differences in these values to the anharmonicity of the systems, which affects the kinetic energy decay method more strongly than the equilibrium correlation analysis:

- Equilibrium correlation analysis
- Kinetic energy decay

Table S13: Comparison of lifetimes from phonon-phonon coupling.

|             | equilibrium correlation analysis |           |           |           | kinetic energy decay |           |           |           |
|-------------|----------------------------------|-----------|-----------|-----------|----------------------|-----------|-----------|-----------|
|             | <b>Lifetime / ps</b>             |           |           |           | <b>Lifetime / ps</b> |           |           |           |
|             | <b>FT</b>                        | <b>FR</b> | <b>SA</b> | <b>IS</b> | <b>FT</b>            | <b>FR</b> | <b>SA</b> | <b>IS</b> |
| sharp tip   | 142.1                            | 69.0      | 56.2      | 48.5      | 138.1                | 20.4      | 14.6      | 17.0      |
| blunt tip   | 110.9                            | 67.0      | 31.9      | 65.4      | 36.4                 | 19.2      | 13.3      | 15.5      |
| slab adatom | 59.8                             | 65.3      | 53.7      | 46.3      | 25.5                 | 14.3      | 15.7      | 21.1      |
| slab        | 19.3                             | 24.6      | 26.8      | 53.7      | 21.7                 | 8.8       | 21.3      | 15.6      |

Electron-phonon lifetimes are calculated in two different ways (see Table S14):

- Quasi-harmonic approximation
- Kinetic energy decay

Table S14: Comparison of lifetimes from electron-phonon coupling.

|             | quasi-harmonic approx. |           |           |           | kinetic energy decay |           |           |           |
|-------------|------------------------|-----------|-----------|-----------|----------------------|-----------|-----------|-----------|
|             | <b>Lifetime / ps</b>   |           |           |           | <b>Lifetime / ps</b> |           |           |           |
|             | <b>FT</b>              | <b>FR</b> | <b>SA</b> | <b>IS</b> | <b>FT</b>            | <b>FR</b> | <b>SA</b> | <b>IS</b> |
| sharp tip   | 187.7                  | 24.7      | 93.6      | 7.7       | 205.5                | 37.4      | 78.3      | 11.1      |
| blunt tip   | 102.3                  | 6.5       | 44.8      | 6.5       | 185.4                | 12.9      | 48.4      | 9.3       |
| slab adatom | 116.2                  | 11.8      | 60.5      | 9.3       | 159.4                | 17.1      | 59.2      | 14.9      |
| slab        | 63.8                   | 4.0       | 13.8      | 3.1       | 105.0                | 7.4       | 19.5      | 6.0       |

Total lifetimes—including effects from electron-phonon and phonon-phonon coupling—are calculated with three different methods (see Table S15):

- Additive relaxation rates: Electron-phonon relaxation rate from quasi-harmonic approximation + phonon-phonon relaxation rate from equilibrium correlation analysis
- Equilibrium correlation analysis
- Kinetic energy decay

Table S15: Comparison of total lifetimes.

|             | additive relaxation rates |           |           |           | equilibrium correlation ana. |           |           |           | kinetic energy decay |           |           |           |
|-------------|---------------------------|-----------|-----------|-----------|------------------------------|-----------|-----------|-----------|----------------------|-----------|-----------|-----------|
|             | <b>Lifetime / ps</b>      |           |           |           | <b>Lifetime / ps</b>         |           |           |           | <b>Lifetime / ps</b> |           |           |           |
|             | <b>FT</b>                 | <b>FR</b> | <b>SA</b> | <b>IS</b> | <b>FT</b>                    | <b>FR</b> | <b>SA</b> | <b>IS</b> | <b>FT</b>            | <b>FR</b> | <b>SA</b> | <b>IS</b> |
| sharp tip   | 80.9                      | 18.2      | 35.1      | 6.7       | 40.4                         | 24.1      | 21.1      | 5.2       | 56.5                 | 17.4      | 12.8      | 6.3       |
| blunt tip   | 53.2                      | 5.9       | 18.6      | 5.9       | 30.0                         | 4.1       | 15.2      | 9.0       | 29.8                 | 6.3       | 11.9      | 5.3       |
| slab adatom | 39.5                      | 10.0      | 28.5      | 7.7       | 21.5                         | 8.5       | 28.4      | 6.3       | 20.9                 | 8.6       | 14.1      | 7.4       |
| slab        | 14.8                      | 3.4       | 9.1       | 3.0       | 19.8                         | 3.6       | 20.7      | 3.6       | 15.9                 | 3.4       | 11.7      | 3.0       |

## S4 Analysis of the velocity cross-correlation function

In the ideal case, the velocity autocorrelation function has the following form:

$$y(t) = \cos(2\pi ft) e^{-t/\tau}, t \geq 0 \quad (2)$$

Here  $f$  is the frequency of the underlying vibration mode and  $\tau$  is its lifetime. We can determine the lifetime by analysing the Fourier transform of  $y(t)$

$$Y(\nu) = \int_0^\infty y(t) e^{-i2\pi\nu t} dt \quad (3)$$

Substituting  $y(t) = \cos(2\pi ft) e^{-t/\tau}$ :

$$Y(\nu) = \int_0^\infty \cos(2\pi ft) e^{-t/\tau} e^{-i2\pi\nu t} dt \quad (4)$$

Using Euler's formula to express  $\cos(2\pi ft)$ :

$$Y(\nu) = \int_0^\infty \frac{1}{2} (e^{i2\pi ft} + e^{-i2\pi ft}) e^{-t/\tau} e^{-i2\pi\nu t} dt \quad (5)$$

Expanding:

$$Y(\nu) = \frac{1}{2} \int_0^\infty e^{t(-\frac{1}{\tau} + i(2\pi f - 2\pi\nu))} dt + \frac{1}{2} \int_0^\infty e^{t(-\frac{1}{\tau} - i(2\pi f + 2\pi\nu))} dt \quad (6)$$

Each term can be integrated separately. For the first term:

$$\int_0^\infty e^{t(-\frac{1}{\tau} + i(2\pi f - 2\pi\nu))} dt = \frac{1}{\frac{1}{\tau} - i(2\pi f - 2\pi\nu)} \quad (7)$$

And for the second term:

$$\int_0^\infty e^{t(-\frac{1}{\tau} - i(2\pi f + 2\pi\nu))} dt = \frac{1}{\frac{1}{\tau} + i(2\pi f + 2\pi\nu)} \quad (8)$$

Thus, the full expression for  $Y(\nu)$  is:

$$Y(\nu) = \frac{1}{2} \left( \frac{1}{\frac{1}{\tau} - i(2\pi f - 2\pi\nu)} + \frac{1}{\frac{1}{\tau} + i(2\pi f + 2\pi\nu)} \right) \quad (9)$$

To separate real and imaginary parts:

$$\text{Re}(Y(\nu)) = \frac{1}{2} \left( \frac{\frac{1}{\tau}}{(\frac{1}{\tau})^2 + (2\pi f - 2\pi\nu)^2} + \frac{\frac{1}{\tau}}{(\frac{1}{\tau})^2 + (2\pi f + 2\pi\nu)^2} \right) \quad (10)$$

$$\text{Im}(Y(\nu)) = \frac{1}{2} \left( \frac{(2\pi f - 2\pi\nu)}{(\frac{1}{\tau})^2 + (2\pi f - 2\pi\nu)^2} - \frac{(2\pi f + 2\pi\nu)}{(\frac{1}{\tau})^2 + (2\pi f + 2\pi\nu)^2} \right) \quad (11)$$

To determine the lifetime, we look at the real positive part of the power spectrum.

$$\text{Re}(Y(\nu+)) = \frac{1}{2} \frac{\frac{1}{\tau}}{\left(\frac{1}{\tau}\right)^2 + (2\pi f - 2\pi\nu)^2} \quad (12)$$

$$= \frac{1}{2} \frac{\frac{1}{\tau}}{\left(\frac{1}{\tau}\right)^2 [1 + (2\pi\tau)^2 (f - \nu)^2]} \quad (13)$$

$$= \frac{1}{2} \frac{1}{\frac{1}{\tau} [1 + (2\pi\tau)^2 (f - \nu)^2]} \quad (14)$$

With  $\gamma = 1/2\pi\tau$  we get a Lorentzian.

$$\text{Re}(Y(\nu+)) = \frac{1}{4\pi\gamma \left[1 + \left(\frac{f-\nu}{\gamma}\right)^2\right]} \quad (15)$$

## S5 Coupling strength between vibrational modes

To estimate coupling strength between vibrational modes from molecular dynamics, we analyse the time-correlated behaviour of the vibrational amplitudes. To understand our analysis, let us consider two weakly coupled vibrational modes  $k$  and  $l$  and assume that the interaction Hamiltonian between modes  $k$  and  $l$  is linear and has the following form.

$$H_{\text{int}} = \lambda q_k q_l, \quad (16)$$

Here  $q_k$  and  $q_l$  are the displacement operators for modes  $k$  and  $l$  and  $\lambda$  is the coupling constant representing the interaction strength between these modes. This Hamiltonian term describes the energy contribution due to the interaction of the two vibrational modes. The coupling constant  $\lambda$  quantifies how strongly the energy of one mode is influenced by the displacement of the other mode. From the Hamiltonian, we can derive equations of motion for the displacements  $q_k$  and  $q_l$ . We use Hamilton's equations to find that the interaction introduces additional terms into the equations of motion of each mode that are proportional to  $\lambda$ .

$$\ddot{q}_k + \omega_k^2 q_k = -\lambda q_l \quad (17)$$

$$\ddot{q}_l + \omega_l^2 q_l = -\lambda q_k \quad (18)$$

Here  $\omega_k$  and  $\omega_l$  are the natural frequencies of modes  $k$  and  $l$ . These coupled equations of motion lead to oscillatory energy exchange between the two modes, with the rate of exchange depending on  $\lambda$ .

### S5.1 Vibrational modes and amplitudes

Suppose we have two vibrational modes  $q_k$  and  $q_l$  with time-dependent amplitudes  $A_k(t)$  and  $A_l(t)$  obtained from an MD trajectory, often through normal mode analysis or Fourier decomposition of atomic displacements. The amplitudes  $A_k(t)$  contain information about the coupling. The displacement for each mode  $q_k$  can be expressed as:

$$q_k(t) = A_k(t) \exp(i\Omega_k t + \phi_k) \quad (19)$$

$$q_l(t) = A_l(t) \exp(i\Omega_l t + \phi_l) \quad (20)$$

Here  $\omega_k$  and  $\omega_l$  are the characteristic frequencies of modes  $k$  and  $l$ .  $\phi_k$  and  $\phi_l$  are the phases. Substituting the vibrational mode solutions in Equation 18 we get.

$$\ddot{A}_k(t) + \tilde{\Omega}_k^2 A_k(t) + \lambda A_l(t) = 0 \quad (21)$$

$$\ddot{A}_l(t) + \tilde{\Omega}_l^2 A_l(t) + \lambda A_k(t) = 0 \quad (22)$$

Here  $\tilde{\Omega}_k^2 = \omega_k^2 - \Omega_k^2$  (same for  $l$ ). To solve the system of coupled differential equations we assume solutions of the form:

$$A_k(t) = A_{k0} e^{i\omega t} \quad (23)$$

$$A_l(t) = A_{l0} e^{i\omega t}. \quad (24)$$

Substituting these into the equations, we get:

$$(-\omega^2 + \tilde{\Omega}_k^2) A_{k0} + \lambda A_{l0} = 0, \quad (25)$$

$$\lambda A_{k0} + (-\omega^2 + \tilde{\Omega}_l^2) A_{l0} = 0. \quad (26)$$

This can be written in matrix form:

$$\begin{pmatrix} \tilde{\Omega}_k^2 - \omega^2 & \lambda \\ \lambda & \tilde{\Omega}_l^2 - \omega^2 \end{pmatrix} \begin{pmatrix} A_{k0} \\ A_{l0} \end{pmatrix} = 0 \quad (27)$$

For non-trivial solutions, the determinant of this matrix must be zero:

$$(\tilde{\Omega}_k^2 - \omega^2)(\tilde{\Omega}_l^2 - \omega^2) - \lambda^2 = 0. \quad (28)$$

Expanding, we obtain:

$$\omega^4 - (\tilde{\Omega}_k^2 + \tilde{\Omega}_l^2)\omega^2 + \tilde{\Omega}_k^2 \tilde{\Omega}_l^2 - \lambda^2 = 0. \quad (29)$$

This is a quadratic equation in  $\omega^2$ , with solutions:

$$\omega^2 = \frac{\tilde{\Omega}_k^2 + \tilde{\Omega}_l^2 \pm \sqrt{(\tilde{\Omega}_k^2 - \tilde{\Omega}_l^2)^2 + 4\lambda^2}}{2}. \quad (30)$$

We can rewrite the eigenvalue equation 30 as follows:

$$\omega^2 = \frac{\tilde{\Omega}_k^2 + \tilde{\Omega}_l^2}{2} \pm \frac{1}{2} \sqrt{(\tilde{\Omega}_k^2 - \tilde{\Omega}_l^2)^2 + 4\lambda^2} \quad (31)$$

For  $\lambda \ll |\tilde{\Omega}_k^2 - \tilde{\Omega}_l^2|$ , we expand the square root term using the binomial expansion:

$$\sqrt{(\tilde{\Omega}_k^2 - \tilde{\Omega}_l^2)^2 + 4\lambda^2} = |\tilde{\Omega}_k^2 - \tilde{\Omega}_l^2| \sqrt{1 + \frac{2\lambda^2}{(\tilde{\Omega}_k^2 - \tilde{\Omega}_l^2)^2}} \approx |\tilde{\Omega}_k^2 - \tilde{\Omega}_l^2| \left( 1 + \frac{2\lambda^2}{(\tilde{\Omega}_k^2 - \tilde{\Omega}_l^2)^2} \right). \quad (32)$$

Substituting this approximation into the expression for  $\omega^2$ , we get for the lower eigenvalue ( $\omega_1^2$ ):

$$\omega_1^2 = \frac{\tilde{\Omega}_k^2 + \tilde{\Omega}_l^2}{2} - \frac{1}{2} \sqrt{(\tilde{\Omega}_k^2 - \tilde{\Omega}_l^2)^2 + 4\lambda^2}. \quad (33)$$

Using the approximation for the square root:

$$\omega_1^2 \approx \frac{\tilde{\Omega}_k^2 + \tilde{\Omega}_l^2}{2} - \frac{1}{2} |\tilde{\Omega}_k^2 - \tilde{\Omega}_l^2| \left( 1 + \frac{2\lambda^2}{(\tilde{\Omega}_k^2 - \tilde{\Omega}_l^2)^2} \right). \quad (34)$$

Simplify:

$$\omega_1^2 \approx \min(\tilde{\Omega}_k^2, \tilde{\Omega}_l^2) - \frac{\lambda^2}{|\tilde{\Omega}_k^2 - \tilde{\Omega}_l^2|}. \quad (35)$$

For the higher eigenvalue ( $\omega_2^2$ ):

$$\omega_2^2 = \frac{\tilde{\Omega}_k^2 + \tilde{\Omega}_l^2}{2} + \frac{1}{2} \sqrt{(\tilde{\Omega}_k^2 - \tilde{\Omega}_l^2)^2 + 4\lambda^2}. \quad (36)$$

Using the approximation for the square root:

$$\omega_2^2 \approx \frac{\tilde{\Omega}_k^2 + \tilde{\Omega}_l^2}{2} + \frac{1}{2} |\tilde{\Omega}_k^2 - \tilde{\Omega}_l^2| \left( 1 + \frac{2\lambda^2}{(\tilde{\Omega}_k^2 - \tilde{\Omega}_l^2)^2} \right). \quad (37)$$

Simplify:

$$\omega_2^2 \approx \max(\tilde{\Omega}_k^2, \tilde{\Omega}_l^2) + \frac{\lambda^2}{|\tilde{\Omega}_k^2 - \tilde{\Omega}_l^2|}. \quad (38)$$

To determine the eigenvectors, we can rewrite equation 27 to get:

$$(\tilde{\Omega}_k^2 - \omega^2)A_{k0} + \lambda A_{l0} = 0 \quad (39)$$

$$\lambda A_{k0} + (\tilde{\Omega}_l^2 - \omega^2)A_{l0} = 0 \quad (40)$$

From the first equation:

$$\frac{A_{k0}}{A_{l0}} = -\frac{\lambda}{\tilde{\Omega}_k^2 - \omega^2}. \quad (41)$$

From the second equation:

$$\frac{A_{l0}}{A_{k0}} = -\frac{\lambda}{\tilde{\Omega}_l^2 - \omega^2}. \quad (42)$$

These two ratios are consistent because:

$$\frac{A_{k0}}{A_{l0}} \cdot \frac{A_{l0}}{A_{k0}} = 1. \quad (43)$$

The eigenvalues are approximately:

$$\omega_1^2 \approx \min(\tilde{\Omega}_k^2, \tilde{\Omega}_l^2) - \frac{\lambda^2}{|\tilde{\Omega}_k^2 - \tilde{\Omega}_l^2|} \quad (44)$$

$$\omega_2^2 \approx \max(\tilde{\Omega}_k^2, \tilde{\Omega}_l^2) + \frac{\lambda^2}{|\tilde{\Omega}_k^2 - \tilde{\Omega}_l^2|}. \quad (45)$$

The eigenvector for  $\omega_1^2$ , the lower Eigenvalue can be calculated by substituting  $\omega_1^2$  into the first equation:

$$(\tilde{\Omega}_k^2 - \omega_1^2)A_{k0} + \lambda A_{l0} = 0. \quad (46)$$

For  $\omega_1^2 \approx \min(\tilde{\Omega}_k^2, \tilde{\Omega}_l^2)$ , we approximate:

$$\tilde{\Omega}_k^2 - \omega_1^2 \approx |\tilde{\Omega}_k^2 - \tilde{\Omega}_l^2|. \quad (47)$$

Thus:

$$\frac{A_{k0}}{A_{l0}} = -\frac{\lambda}{\tilde{\Omega}_k^2 - \omega_1^2} \approx -\frac{\lambda}{|\tilde{\Omega}_k^2 - \tilde{\Omega}_l^2|}. \quad (48)$$

The eigenvector is then:

$$\mathbf{v}_1 = \begin{pmatrix} 1 \\ -\frac{\lambda}{|\tilde{\Omega}_k^2 - \tilde{\Omega}_l^2|} \end{pmatrix}. \quad (49)$$

We can determine the eigenvector for  $\omega_2^2$ , the higher eigenvalue, by substituting  $\omega_2^2$  into the first equation:

$$(\tilde{\Omega}_k^2 - \omega_2^2)A_{k0} + \lambda A_{l0} = 0. \quad (50)$$

For  $\omega_2^2 \approx \max(\tilde{\Omega}_k^2, \tilde{\Omega}_l^2)$ , we approximate:

$$\tilde{\Omega}_k^2 - \omega_2^2 \approx -|\tilde{\Omega}_k^2 - \tilde{\Omega}_l^2|. \quad (51)$$

Thus:

$$\frac{A_{k0}}{A_{l0}} = -\frac{\lambda}{\tilde{\Omega}_k^2 - \omega_2^2} \approx \frac{\lambda}{|\tilde{\Omega}_k^2 - \tilde{\Omega}_l^2|}. \quad (52)$$

The eigenvector is then:

$$\mathbf{v}_2 = \begin{pmatrix} 1 \\ \frac{\lambda}{|\tilde{\Omega}_k^2 - \tilde{\Omega}_l^2|} \end{pmatrix}. \quad (53)$$

These solutions correspond to two normal mode frequencies,  $\omega_1$  and  $\omega_2$ , which describe the coupled oscillations of  $A_k$  and  $A_l$ .

$$A_k(t) = A_{k0}e^{-i\omega_1 t} + A'_{k0}e^{-i\omega_2 t} \quad (54)$$

$$A_l(t) = A_{l0}e^{-i\omega_1 t} + A'_{l0}e^{-i\omega_2 t} \quad (55)$$

The influence of the coupling constant  $\lambda$  on the dynamics is reflected in the cross-correlation function  $C_{kl}(t) = \langle A_k(t)A_l(0) \rangle$ . Since  $\lambda$  mixes the motion of  $A_k$  and  $A_l$ , it will affect the amplitude and phase relationships between them. The presence of  $\lambda$  leads to oscillations in  $C_{kl}(t)$  at the combined normal mode frequencies  $\omega_1$  and  $\omega_2$ , showing energy exchange between the modes  $A_k$  and  $A_l$  due to coupling.

## S5.2 Cross-correlation function

To obtain the coupling strength  $\lambda$  we calculate the Fourier transform of the cross-correlation function  $C_{kl}(t)$ . The cross-correlation function  $C_{kl}(t)$  is defined as follows:

$$C_{kl}(t) = \langle A_k(t)A_l(0) \rangle \quad (56)$$

Here  $A_k(t)$  and  $A_l(t)$  are the time-dependent amplitudes of the vibration modes, and  $\langle \dots \rangle$  denotes an average over the ensemble. The Fourier transform of the cross-correlation function  $C_{kl}(t)$  is given by:

$$\tilde{C}_{kl}(\omega) = \int_{-\infty}^{\infty} C_{kl}(t) e^{-i\omega t} dt. \quad (57)$$

We substitute the solutions for the normal modes from Equation 55 into the cross-correlation function. Note that  $\lambda$  influences the amplitudes  $A_{k0}$  and  $A_{l0}$ .

$$C_{kl}(t) = \langle (A_{k0} e^{-i\omega_1 t} + A'_{k0} e^{-i\omega_2 t})(A_{l0} + A'_{l0}) \rangle. \quad (58)$$

From the eigenvectors, we know that:

$$A_{k0} \approx A_{l0} \frac{\lambda}{|\tilde{\Omega}_k^2 - \tilde{\Omega}_l^2|} \quad (59)$$

Therefore the cross-correlation function can be approximated as follows:

$$C_{kl}(t) \propto \frac{\lambda}{|\tilde{\Omega}_k^2 - \tilde{\Omega}_l^2|} (e^{-i\omega_1 t} + e^{-i\omega_2 t}) \quad (60)$$

When taking the Fourier transform of  $C_{kl}(t)$ , we find contributions from both  $\omega_1$  and  $\omega_2$ . The resulting expression can be analysed in terms of the amplitudes and their relationship to the coupling strength  $\lambda$ . The coupling strength can be obtained from the Fourier coefficients of the cross-correlation function:

$$\tilde{C}_{kl}(\omega) \propto \frac{\lambda}{\omega^2 - \omega_1^2} + \frac{\lambda}{\omega^2 - \omega_2^2}, \quad (61)$$

leading to:

$$\lambda \propto \left. \frac{\tilde{C}_{kl}(\omega)}{\omega^2 - \omega_i^2} \right|_{\omega=\omega_i}, \quad (i = 1, 2). \quad (62)$$

This means that by analysing the peak values of the Fourier transform at the frequencies corresponding to the normal modes, you can estimate  $\lambda$ . The height of the peaks  $\tilde{C}_{kl}(\omega)|_{\omega=\omega_{1/2}}$  is related to the coupling strength.

### S5.3 Coupling strength between vibration modes

We visualise the coupling density  $\rho_j(\omega)$  between a given CO mode and the other modes in the system:

$$\rho_j(\omega) = \sum_i \tilde{C}_{ij}(\omega) \quad (63)$$

A comparison of the coupling density with and without electron-phonon interaction reveals that the coupling is significantly stronger when electron-phonon coupling is included. We observe the strongest coupling for the FR and IS modes. The geometry of the surface significantly affects the coupling density: The sharp tip exhibits the smallest coupling, while the slab shows the largest.

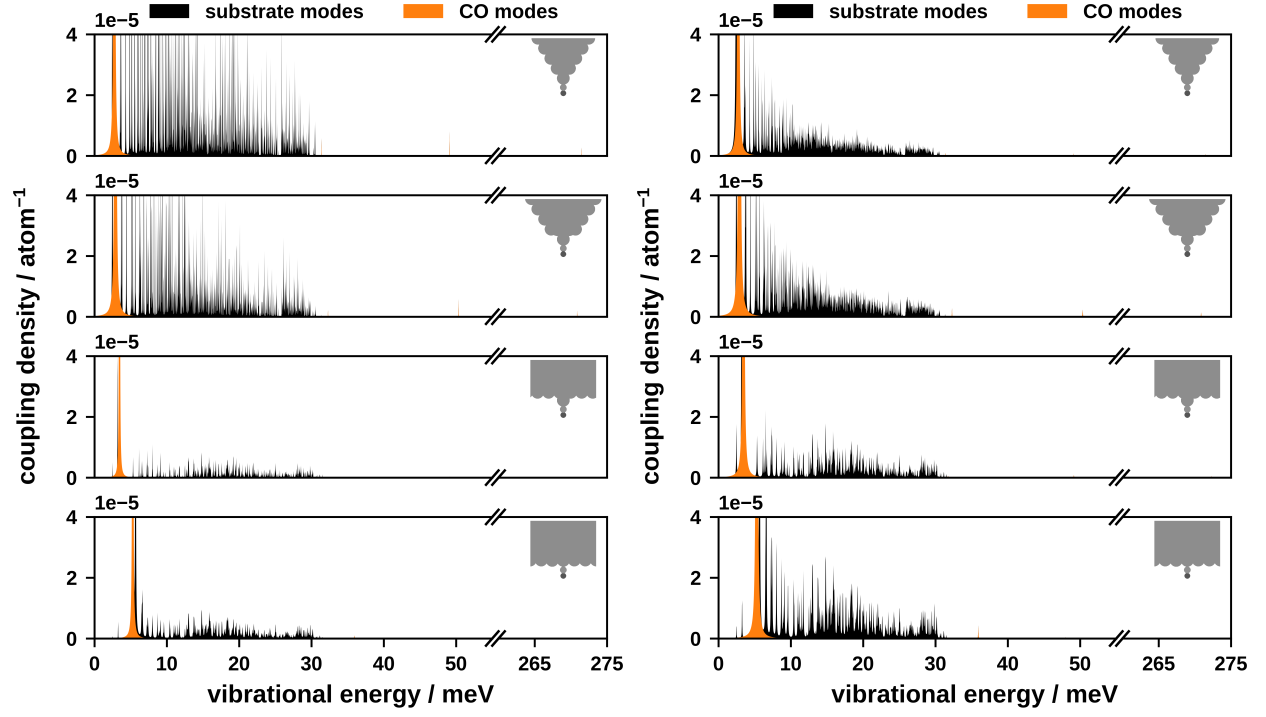

Figure S18: Coupling density of the FT mode with all other modes; Left) phonon-phonon coupling only; Right) electron-phonon and phonon-phonon coupling.

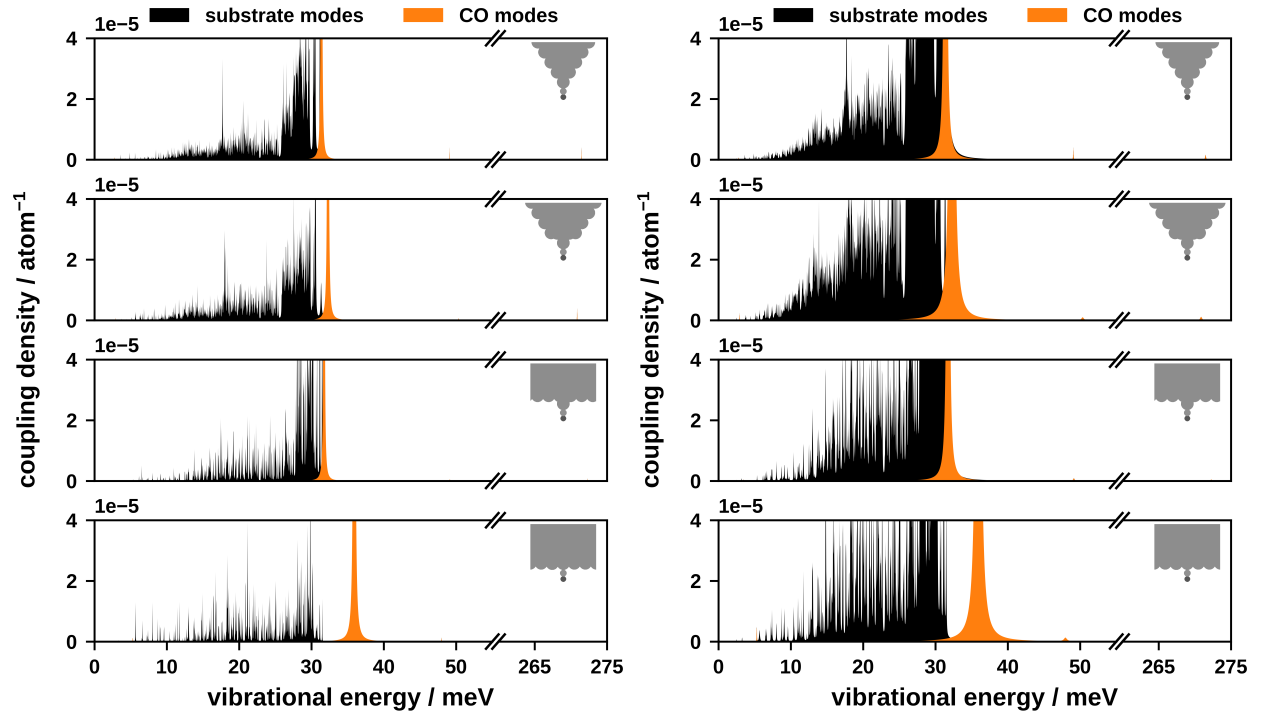

Figure S19: Coupling density of the FR mode with all other modes; Left) phonon-phonon coupling only; Right) electron-phonon and phonon-phonon coupling.

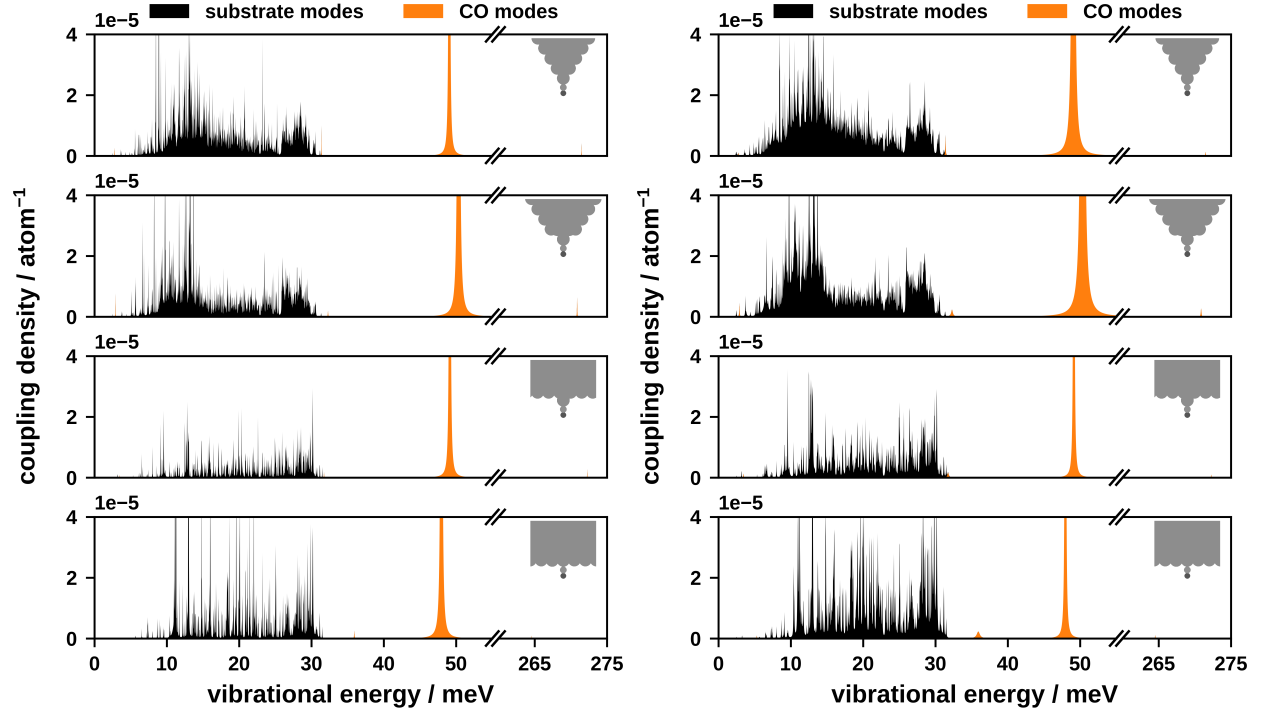

Figure S20: Coupling density of the SA mode with all other modes; Left) phonon-phonon coupling only; Right) electron-phonon and phonon-phonon coupling.

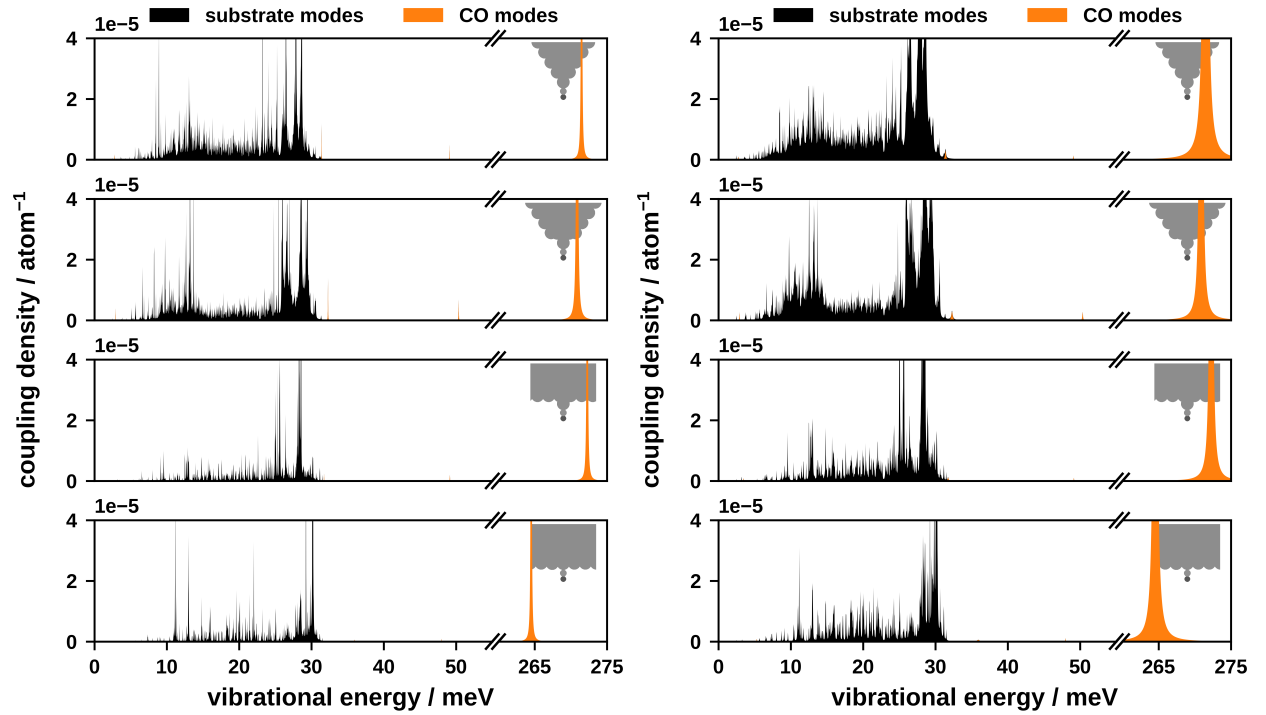

Figure S21: Coupling density of the IS mode with all other modes; Left) phonon-phonon coupling only; Right) electron-phonon and phonon-phonon coupling.

## References

- (1) Blum, V.; Gehrke, R.; Hanke, F.; Havu, P.; Havu, V.; Ren, X.; Reuter, K.; Scheffler, M. Ab initio molecular simulations with numeric atom-centered orbitals. *Comput. Phys. Commun.* **2009**, *180*, 2175–2196.
- (2) Feibelman, P. J.; Hammer, B.; Nørskov, J. K.; Wagner, F.; Scheffler, M.; Stumpf, R.; Watwe, R.; Dumesic, J. The co/pt (111) puzzle. *The Journal of Physical Chemistry B* **2001**, *105*, 4018–4025.
- (3) Hu, Q.-M.; Reuter, K.; Scheffler, M. Towards an Exact Treatment of Exchange and Correlation in Materials: Application to the “CO Adsorption Puzzle” and Other Systems. *Phys. Rev. Lett.* **2007**, *98*, 176103.
- (4) Kessler, J.; Thieme, F. Chemisorption of CO on differently prepared Cu(111) surfaces. *Surf. Sci.* **1977**, *67*, 405–415.
- (5) Vollmer, S.; Witte, G.; Wöll, C. Determination of site specific adsorption energies of CO on copper. *Catalysis letters* **2001**, *77*, 97–101.
- (6) Eren, B.; Zherebetskyy, D.; Patera, L. L.; Wu, C. H.; Bluhm, H.; Africh, C.; Wang, L.-W.; Somorjai, G. A.; Salmeron, M. Activation of Cu (111) surface by decomposition into nanoclusters driven by CO adsorption. *Science* **2016**, *351*, 475–478.
- (7) Braun, J.; Graham, A. P.; Hofmann, F.; Silvestri, W.; Toennies, J. P.; Witte, G. A He-atom scattering study of the frustrated translational mode of CO chemisorbed on defects on copper surfaces. *J. Chem. Phys.* **1996**, *105*, 3258–3263.
- (8) Hirschmugl, C. J.; Williams, G. P. Chemical shifts and coupling interactions for the bonding vibrational modes for CO/Cu (111) and (100) surfaces. *Phys. Rev. B* **1995**, *52*, 14177.
- (9) Batatia, I.; Kovacs, D. P.; Simm, G.; Ortner, C.; Csányi, G. MACE: Higher order equivariant message passing neural networks for fast and accurate force fields. *Advances in Neural Information Processing Systems* **2022**, *35*, 11423–11436.
